# Supplementary material for: Deformation enduring conveyance of structured light through multimode waveguides and its exploitation for flexible hair-thin endoscopes
Source: arXiv:2512.23514 ancillary file (2025-12-29)
Supplement: Supplementary file 1 [file Suppl_Materials.pdf]

# Supplementary Materials for

## Deformation enduring conveyance of structured light through multimode waveguides and its exploitation for flexible hair-thin endoscopes

Sergey Turtaev†, Tomáš Tyc†, Ulf Poßner, Tina Eschrich, Torsten Poßner, Yang Du, André Gomes, Bernhard Messerschmidt, and Tomáš Čižmár
Correspondence to: tomas.cizmar@leibniz-ipht.de

**This PDF file includes:**

Materials and Methods
Figs. S1 to S9
Table S1
Captions for Movies SM1 to SM5
Caption for Data S1

**Other Supplementary Materials for this manuscript include the following:**

Movies SM1 to SM5
Data S1 to S2 [FibreBendingDesigns.zip, DataArchive.zip]

**Materials and Methods**

1. <u>Finding modes of a bent GRIN fibre with a perturbation of the refractive index</u>

In our experiments we used a GRIN fibre whose refractive index profile is close to the ideal parabolic one, but not perfect. The 2D index profile $n(x, y)$ in a selected cross section of the fibre was measured as explained in the main article, and the resulting squared profile was fitted by the ideal parabolic profile

$$n_{\mathrm{id}}^2(x, y) = n_0^2\left(1 - \frac{x^2 + y^2}{b^2}\right), \qquad (S6)$$

where the parameters $n_0$ and $b$ characterise the refractive index on the fibre axis and index steepness, respectively. The square of the measured 2D index profile can then be expressed as a sum of the ideal profile and the index perturbation

$$n^2(x, y) = n_{\mathrm{id}}^2(x, y) + \Delta n^2(x, y)\,. \qquad (S7)$$

We want to describe light propagation in the fibre whose refractive index is perturbed like this and it is bent at the same time. To do so, we start from the exact equation for the transverse part of the electric field $\mathbf{e}_{\mathrm{t}}$ in a straight fibre[1]

$$[\nabla_{\mathrm{t}}^2 + k^2 n^2 - \beta^2]\mathbf{e}_{\mathrm{t}} = -\nabla_{\mathrm{t}}(\mathbf{e}_{\mathrm{t}} \cdot \nabla_{\mathrm{t}} \ln\, n^2)\,, \qquad (S8)$$

where $\nabla_{\mathrm{t}}$ is the transverse nabla operator. In a bent fibre the local phase velocity of the wave is not constant throughout the fibre cross section but depends linearly on the distance from the centre of curvature[1,2]. If we assume that the fibre is bent in the $x$ direction and has curvature $\rho$, this corresponds to replacing $\beta^2$ in Eq. S8 by the expression $[\beta/(1-\rho x)]^2 \approx \beta^2 + 2\beta^2\rho x$. In normal conditions, the second term $2\beta^2\rho x$ is smaller than the first term $\beta^2$ by several orders of magnitude. Then we can take advantage of the fact that the propagation constant of all the guided modes belong to a narrow range, $\beta \in (kn_{\mathrm{cl}}, kn_0)$, where $n_{\mathrm{cl}}$ is the refractive index of the cladding. This enables to replace $\beta$ in the second term by $kn_0$, so we finally get $[\beta/(1-\rho x)]^2 \approx \beta^2 + 2k^2 n_0^2 \rho x$. With this modification to Eq. S8 and upon employing Eq. S7, we get

$$\left[\nabla_{\mathrm{t}}^2 + k^2(n_{\mathrm{id}}^2 + \Delta n^2 - 2n_0^2\rho x) - \beta^2\right]\mathbf{e}_{\mathrm{t}} = -\nabla_{\mathrm{t}}(\mathbf{e}_{\mathrm{t}} \cdot \nabla_{\mathrm{t}} \ln\, n^2)\,. \qquad (S9)$$

Next we expand the transverse field into a suitable basis of states. Such a basis can be derived from the basis of solutions of the scalar Helmholtz equation for the ideal parabolic index profile,

$$\left[\Delta_{\mathrm{t}} + k^2 n_{\mathrm{id}}^2 - \beta_{0i}^2\right]\psi_i = 0\,, \qquad (S10)$$

where $\beta_{0i}$ are the scalar propagation constants and $\psi_i$ are the Laguerre-Gauss modes[1,2]. The basis for the transverse electric field $\mathbf{e}_{\mathrm{t}}$ will then consist of the states $\psi_i$ equipped with a unit polarisation vector $\hat{\mathbf{e}}_p$, where index $p$ denotes one of two possible linear polarisation states $p \in \{\mathrm{x}, \mathrm{y}\}$. This way, we expand the field as

$$\mathbf{e}_\mathrm{t} = \sum_{i=1}^{N} \sum_{p\in\{x,y\}} c_{ip}\, \psi_i(x,y)\, \hat{\mathbf{e}}_p\,, \tag{S11}$$

where $N$ is the number of scalar modes that are guided by the fibre, so there are $2N$ states in our vector basis. Next we substitute this expansion into Eq. (S9), use Eq. (S10), multiply the resulting equation by $\hat{\mathbf{e}}_q\psi_j^*$, where $\mathrm{q} \in \{\mathrm{x,y}\}$ describes the linear polarisation we are projecting to, and integrate over the plane $xy$. Using in addition the orthonormality of the set of the scalar modes $\psi_i$, we get

$$c_{jq}\left(\beta_{0j}^2 - \beta^2\right) + \sum_i c_{iq} k^2 \int_{\mathbb{R}^2} \psi_j^*(\Delta n^2 - 2n_0^2\rho x)\psi_i \,\mathrm{d}x\,\mathrm{d}y =$$
$$-\sum_{ip} c_{ip} \int_{\mathbb{R}^2} \psi_j^*\hat{\mathbf{e}}_q \cdot \nabla_\mathrm{t}\left(\psi_i\hat{\mathbf{e}}_p \cdot \nabla_\mathrm{t} \ln n^2\right) \mathrm{d}x\,\mathrm{d}y\,. \tag{S12}$$

The next step is to simplify the integral on the right-hand side. For this purpose, to shorten the expressions, we introduce the scalar functions $P_{ip} = (\psi_i\hat{\mathbf{e}}_p \cdot \nabla_\mathrm{t}\ln\, n^2)$, and write the integral as

$$\int_{\mathbb{R}^2} \psi_j^*\hat{\mathbf{e}}_q \cdot \left(\nabla_\mathrm{t} P_{ip}\right) dxdy = \int_{\mathbb{R}^2} \nabla_\mathrm{t} \cdot \left(\psi_j^*\hat{\mathbf{e}}_q P_{ip}\right) dxdy - \int_{\mathbb{R}^2} P_{ip} \nabla_\mathrm{t} \cdot \left(\psi_j^*\hat{\mathbf{e}}_q\right) \mathrm{d}x\,\mathrm{d}y \tag{S13}$$

Next we take advantage of the fact that the integral over a 2D area $A$ can be transformed into a line integral,

$$\int_A \nabla_\mathrm{t} \cdot (\psi_j^*\hat{\mathbf{e}}_q P_{ip})\, dxdy = \int_l (\psi_j^*\hat{\mathbf{e}}_q P_{ip}) \cdot \hat{\mathbf{n}}\, dl\,, \tag{S14}$$

see e.g. Eq. (37-55) of [1]. Here the line $l$ encircles the area $A$ and $\hat{\mathbf{n}}$ denotes the unit outward normal to the line element $dl$. Now, expanding the area $A$ to infinity, the line integral vanishes due to the exponential decay of the fields $\psi_j$ and $P_{ip}$. This way, only the second term on the right-hand side of Eq. (S13) is nonzero. Substituting Eq. (S13) into Eq. (S12) then yields

$$c_{jq}\left(\beta_{0j}^2 - \beta^2\right) + \sum_i c_{iq} k^2 \int_{\mathbb{R}^2} \psi_j^*(\Delta n^2 - 2n_0^2\rho x)\psi_i \,\mathrm{d}x\,\mathrm{d}y$$
$$-\sum_{ip} c_{ip} \int_{\mathbb{R}^2} \hat{\mathbf{e}}_q \cdot \left(\nabla_\mathrm{t}\psi_j^*\right)\psi_i\left(\hat{\mathbf{e}}_p \cdot \nabla_\mathrm{t} \ln n^2\right) \mathrm{d}x\,\mathrm{d}y = 0\,. \tag{S15}$$

This equation can be expressed in a matrix form as $\hat{B}^2\mathbf{c} = \beta^2\mathbf{c}$, where $\mathbf{c}$ is a column vector of the coefficients $c_{ip}$ and $\hat{B}^2$ is a $2N \times 2N$ matrix

$$\hat{B}^2 = \hat{B}_0^2 + k^2\hat{M} - 2k^2 n_0^2 \rho \hat{X} - \hat{G}\,. \tag{S16}$$

Here the matrices $\hat{B}_0^2, \hat{M}, \hat{X}$ and $\hat{G}$ are indexed by index pairs $ip$ and $jq$ and their entries are

$$(\hat{B}_0^2)_{jq,ip} = \delta_{ji}\delta_{qp}\beta_{0i}^2 \qquad (S17)$$

$$(\hat{M})_{jq,ip} = \delta_{qp}\int_{\mathbb{R}^2} \Delta n^2 \psi_j^* \psi_i \,\mathrm{d}x\,\mathrm{d}y \qquad (S18)$$

$$(\hat{X})_{jq,ip} = \delta_{qp}\int_{\mathbb{R}^2} x \psi_j^* \psi_i \,\mathrm{d}x\,\mathrm{d}y \qquad (S19)$$

$$(\hat{G})_{jq,ip} = \int_{\mathbb{R}^2} \hat{\mathbf{e}}_q \cdot (\nabla_{\mathrm{t}} \psi_j^*) \psi_i (\hat{\mathbf{e}}_p \cdot \nabla_{\mathrm{t}} \ln n^2) \,\mathrm{d}x\,\mathrm{d}y\,. \qquad (S20)$$

The effects of index perturbation, bending and spin-orbit interaction are described by the matrices $\hat{M}, \hat{X}$ and $\hat{G}$, respectively.

To employ our calculation practically, we calculate, for a given fibre, first the scalar modes and their propagation constants $\beta_{0i}$. We then numerically calculate the matrices $\hat{B}_0^2, \hat{M}, \hat{X}$ and $\hat{G}$. For a given curvature $\rho$, we then calculate the matrix $\hat{B}^2$ via Eq. S16 and subsequently its square root that we denote by $\hat{B} = (\hat{B}^2)^{1/2}$. Since the entries of the matrices $\hat{M}, \hat{X}$ and $\hat{G}$ are very small compared to the diagonal entries of $\hat{B}_0^2$ that are positive real numbers, such a matrix square root can be defined uniquely, taking the branch cut of the complex square root function along the negative real axis.

The matrix $\hat{B}$ describes light propagation in the bent fibre with perturbed refractive index. In particular, the eigenvalues of $\hat{B}$ are columns of coefficients $c_{jq,ip}$ that correspond to the modes of the fibre expressed as superpositions of our basis states. Moreover, the eigenvalues of $\hat{B}$ describe the propagation constants of these modes. This way, the operator describing the evolution of the state in the fibre of length $l$ can simply be expressed as $\hat{U}_\rho(l) = \exp(i\hat{B}l)$ in our basis.

To describe the evolution in the fibre that is not bent uniformly but whose curvature changes along its length, we divide it in a sufficient number of segments (in out calculations we used 100 segments), each of length $\Delta l$, the curvature in each of which can be regarded as constant. Then we simply multiply the matrices $\hat{U}_\rho(\Delta l)$ for the subsequent segments, which yields the total evolution operator.

In our experiments the fibre was bent in different directions, not just the $x$ direction. To describe bending in the direction that makes an angle $\theta$ with the $x$ axis, we must replace the matrix $\hat{X}$ of Eq. S19 by a matrix $\hat{X}_\theta$ defined analogously, but with $x$ replaced by $x_\theta = x\cos\theta + y\sin\theta$ in Eq. S19. The matrix $\hat{X}_\theta$ can be obtained from the matrix $\hat{X}$ by employing the rotation operator $\hat{R}_\theta$ that rotates any state by the angle $\theta$, such that $\hat{X}_\theta = \hat{R}_\theta \hat{X} \hat{R}_\theta^\dagger$.

In our experiments we worked with circularly polarised states rather than linearly polarised ones, while the calculation above employs the latter basis for the sake of simplicity. Transforming any matrix from one basis to the other is given by a simple similarity transformation.

2. Influence of odd and even perturbations of the refractive index on the modes

For a 'naïve' ray-optics based explanation of this phenomenon, see Supplementary movie SM5.

As we have shown, refractive index perturbation $\Delta n^2$ influence the modes via the matrix elements $(\hat{M})_{jq,ip}$ given by Eq. (S18) while fibre bending is related to the elements $(\hat{X})_{jq,ip}$ of Eq. (S19). To see some specific features of the situation when both the index perturbation and bending are present, we use a slightly different approach.

To do this, we consider an unperturbed fibre bent in the positive $x$ direction as the starting point, and add the index perturbation on top of that. Then we can repeat the procedure described in Sec.1 of this document, but with the modes of a straight fibre $\psi_i$ replaced by the modes of a bent fibre that we can denote by $\psi'_i$. The effect of the index perturbation will then be described by matrix elements analogous to Eq. (S18):

$$\hat{M}'_{jq,ip} = \delta_{pq} \int_{\mathbb{R}^2} {\psi_j}'^*(x,y){\psi_i}'(x,y)\Delta n^2 \, \mathrm{d}x \, \mathrm{d}y. \quad (S21)$$

As it is well known[2], the modes are, with a good precision, the same as the modes of a straight fibre, just shifted by a certain distance $\Delta x$ in the negative $x$ direction (i.e., toward the outer side of the bend), so we can write approximately

$$\psi_i'(x,y) = \psi_i(x + \Delta x, y) \approx \psi_i(x,y) + \frac{\partial \psi_i(x,y)}{\partial x}\Delta x. \quad (S22)$$

To shorten the notation, we denote the product that appears in Eq. $(S21)$ as

$$\rho'_{ji}(x,y) \equiv \psi_j'^*(x,y)\psi_i'(x,y), \quad (S23)$$

for which we can write a similar equation as $(S22)$:

$$\rho'_{ji}(x,y) = \rho_{ji}(x,y) + \frac{\partial \rho_{ji}(x,y)}{\partial x}\Delta x, \quad (S24)$$

where $\rho_{ji}(x,y) \equiv \psi_j^*(x,y)\psi_i'(x,y)$ corresponds to the modes of a straight fibre.

Now we investigate the effect of adding the index perturbation to the ideal bent fibre. For a weak perturbation, the first order perturbation theory provides a good approximation. In the nondegenerate case, the perturbation corrections to the squared propagation constants would simply be described by diagonal elements of the matrix $M'$ multiplied by $k^2$; however, in the ideal parabolic fibre, even when it is bent, there is a strong degeneracy of the modes, and one must diagonalise the perturbation within the degenerate subspaces first. This corresponds to choosing the "right" eigenvectors from the degenerate subspaces to which the actual bent fibre modes converge when the index perturbation gradually weakens and finally disappears. Without loss of generality, we can assume that the modes $\psi_i'$ (and similarly their straight-fibre counterparts $\psi_i$) have already been chosen this way. Then, the deviations of squared propagation constants $\beta^2$,

compared to the situation without index perturbation, correspond to the diagonal elements of the matrix $M'$ multiplied by $k^2$ similarly as in the non-degenerate case.

We can now evaluate these diagonal matrix elements corresponding to a bent perturbed fibre. To do that, we substitute Eq. $(S24)$into Eq. $(S21)$:

$$M'_{iq,ip} = \delta_{pq} \int_{\mathbb{R}^2} \rho'_{ii}(x,y) \Delta n^2(x,y)\, \mathrm{d}x\, \mathrm{d}y = M'^{(0)}_{iq,ip} + \Delta x \delta_{pq} \int_{\mathbb{R}^2} \frac{\partial \rho_{ii}(x,y)}{\partial x} \Delta n^2(x,y)\, \mathrm{d}x\, \mathrm{d}y. \quad (S25)$$

Here $M'^{(0)}_{iq,ip}$ is the matrix element of the index perturbation evaluated for the straight fibre. We will now compare the effect of the perturbation for bent fibre with its effect for the straight fibre; the difference between the two effects is given by the term with the integral on the RHS of Eq. $(S25)$. In the ideal parabolic fibre, the scalar propagation constants depend only on the combination $|l| + 2p$ of the mode indexes $l$ (the angular momentum index) and $p$ (the radial function index)[2]. This means that the $l$ indexes for the degenerate modes always differ by an even number, so each of the modes $\psi_i$ contains only components of the same parity of l. Since the angular part of the mode with a given $l$, i.e., $\mathrm{e}^{\mathrm{i}l\phi}$, is an odd function for $l$ odd and an even function for $l$ even, we see that each "right mode" $\psi_i$ must be an even function for l even (i.e., $\psi_i(-x,-y) = \psi_i(x,y)$) and an odd function for l odd (i.e., $\psi_i(-x,-y) = -\psi_i(x,y)$). Consequently, $\rho_{ii}(x,y)$ must always be an even function and the partial derivative in Eq. $(S25)$ must hence be an odd function.

Now assume that the index perturbation $\Delta n^2(x,y)$ is even, i.e. $\Delta n^2(-x,-y) = \Delta n^2(x,y)$. The function in the integral in Eq. $(S25)$ is then an odd function because it is a product of an odd and even function. The integral therefore vanishes and we find that $M'_{iq,ip} = M'^{(0)}_{iq,ip}$. This means that the effect of an even perturbation on the bent fibre described by $M'_{iq,ip}$ is essentially the same as the effect of the perturbation on the straight fibre described by $M'^{(0)}_{iq,ip}$. Note that this does not mean that there would be no effect of the even perturbation on the fibre modes. The effect does exist, but since we are calibrating the perturbed (albeit straight) fibre, the imaging is not degraded. If, on the other hand, the function $\Delta n^2(x,y)$ is odd, i.e. $\Delta n^2(-x,-y) = -\Delta n^2(x,y)$, then the integrand on the RHS of Eq. $(S25)$ is an even function, and the integral is nonzero in general. Therefore, odd index perturbations have different effects on a bent and straight fibre, and hence they degrade the imaging upon bending.

3. Influence of fibre radius and NA

Eq. $(S25)$ enables us to estimate how the influence of index perturbations changes when we change the fibre radius and numerical aperture. For this purpose, we perform integration by parts with respect to $x$ in Eq.$(S25)$ , obtaining

$$\int_{\mathbb{R}^2} \frac{\partial \rho_{ii}}{\partial x} \Delta n^2\, \mathrm{d}x\, \mathrm{d}y = \int_{\mathbb{R}^2} (\rho_{ii} \Delta n^2) \Big|_{x=-\infty}^{x=\infty} \mathrm{d}y - \int_{\mathbb{R}^2} \rho_{ii} \frac{\partial \Delta n^2(x,y)}{\partial x} \mathrm{d}x\, \mathrm{d}y. \quad (S26)$$

Due to the exponential decay of the modes for large radii, the first term vanishes and only the second term remains, so we can rewrite Eq. $(S25)$ as

$$M'_{iq,ip} - M'^{(0)}_{iq,ip} = -\delta_{pq}\Delta x \int_{\mathbb{R}^2} \rho_{ii} \frac{\partial \Delta n^2(x,y)}{\partial x} \mathrm{d}x\, \mathrm{d}y. \qquad (S27)$$

Suppose now that the NA of the fibre is fixed and the radius $R$ is varied while the index perturbation keeps its functional form (e.g., it is one of the Zernike functions) that is spread over the fibre radius $R$; in other words, the perturbation can be expressed as $\Delta n^2(x,y) = f\left(\frac{x}{R}, \frac{y}{R}\right)$, where $f$ is a fixed function. Then the partial derivative $\frac{\partial \Delta n^2(x,y)}{\partial x}$ in Eq. $(S25)$ scales like $R^{-1}$ and since the modes are normalised, $\int_{\mathbb{R}^2} \rho_{ii}\, \mathrm{d}x\, \mathrm{d}y = 1$, so does scale the whole integral. On the other hand, if we instead fix the fibre radius $R$ and change the numerical aperture, the partial derivative $\frac{\partial \Delta n^2(x,y)}{\partial x}$ does not change, so the integral in Eq. $(S27)$ changes either. The last thing that remains to take into account is the dependence on R and NA of the mode shift $\Delta x$ caused by the bending. It can be shown[2] that the shift is given approximately by $\Delta x = \rho b^2 = \frac{\rho n_0^2 R^2}{NA^2}$. Combining in Eq. $(S27)$ the dependences on $R$ and $NA$ of $\Delta x$ and the integral, we get

$$M'_{iq,ip} - M'^{(0)}_{iq,ip} \propto \frac{R^2}{NA^2}\frac{1}{R} = \frac{R}{NA^2}.$$

This way, the index perturbation influence on imaging performance scales proportionally to the fibre radius and inversely proportionally to the square of the fibre numerical aperture.

4. Adiabatic shapes of fibre probe under bending

In our experiments we used fibre shapes for which the curvature changes smoothly all the way from proximal to distal end. This way the fibre modes that are influenced by the fibre curvature change smoothly as well and the state of light adiabatically adapts to the changing conditions. The imaging performance is therefore less degraded than for non-adiabatic changes of the curvature, which is desirable.

Since both fibre ends are inserted in rigid ferrules, the curvature at the ends is zero. We therefore look for an equilibrium fibre shape satisfying these boundary conditions, which corresponds to zero torque within the fibre at the ends. To find the fibre shape, we follow the procedure described in Ref. [3]. We assume that the deformation occurs only in one plane which we take as the $xy$ plane, and that the force $\vec{F}$ with which adjacent elements of the fibre act on each other is oriented along the $x$ axis.

Further, let $\theta$ denote the angle between the axis of a fibre element located at the point $(x,y)$ and the $x$ axis, $E$ and $I$ denote the Young elastic module and the moment of inertia of the fibre cross section (i.e., a disk), respectively, and let $l$ be the length measured along the fibre. We then arrive at the following differential equation[3] for $\theta$,

$$EI\frac{d^2\theta}{dl^2} - F\sin\,\theta = 0\,. \qquad (S28)$$

This equation, when multiplied by $d\theta/dl$, can be integrated to obtain $EI\ (d\theta/dl)^2/2 + F\cos\ \theta = A$, where $A$ is a constant. From this we express the derivative

$$\frac{d\theta}{dl} = \sqrt{\frac{2(A - F\cos\ \theta)}{EI}} \tag{S29}$$

that expresses the curvature and has to be zero at both ends of the bent fibre segment, which implies that $A = F\cos\ \theta$ (at both ends), i.e., at $l = 0$ and $l = L$, where $L$ is the total length of the fibre segment between the ferrules, which experiences bending. If we denote by $\theta_0$ the value of $\theta$ corresponding to $l = 0$, we can write $\theta_0 = \arccos\ (A/F)$, and the length of the fibre is

$$L = \sqrt{\frac{EI}{2}} \int_{\theta_0}^{2\pi-\theta_0} \frac{d\theta}{\sqrt{A - F\cos\ \theta}} = \sqrt{\frac{EI}{2F}} \int_{\theta_0}^{2\pi-\theta_0} \frac{d\theta}{\sqrt{\cos\ \theta_0 - \cos\ \theta}}\ . \tag{S30}$$

The upper limit $2\pi - \theta_0$ corresponds to the smallest value of $\theta > \theta_0$ where the zero-curvature condition, $A = F\cos\ \theta$, is again satisfied. This way, the angle between the directions of the fibre at its two ends is $\Delta\theta = 2\pi - \theta_0 - \theta_0 = 2(\pi - \theta_0)$.

Further, with the help of Eq. (S29) we can express the coordinates $x, y$ as functions of $\theta$, which describes the fibre shape parametrically:

$$x = \int_0^l \cos\ \theta\ dl = \sqrt{\frac{EI}{2F}} \int_{\theta_0}^{\theta} \frac{\cos\theta\ d\theta}{\sqrt{\cos\theta_0 - \cos\theta}}\ , \tag{S31}$$

and

$$y = \int_0^l \sin\ \theta\ dl = \sqrt{\frac{EI}{2F}} \int_{\theta_0}^{\theta} \frac{\sin\theta\ d\theta}{\sqrt{\cos\theta_0 - \cos\theta}} = \sqrt{\frac{2EI}{F}} \sqrt{\cos\theta_0 - \cos\theta}\ . \tag{S32}$$

These equations fully determine the fibre shape in a parametric way, but they still contain constants $E, I, F$ that might not be easy to access experimentally. However, in an experiment we can easily access the fibre length $L$ and the angle $\Delta\theta$ defined above. To employ them, we first calculate $\theta_0$ from the known $\Delta\theta$ and evaluate the integral in Eq. (S30) which, together with the known value of $L$, determines the constant $\sqrt{EI/F}$. Equipped with its value, we solve equation (S28) numerically to determine the function $\theta_1$, and subsequently use the parametric equations (S31) and (S32) to find the fibre shape $(x(\theta), y(\theta))$ as well as the fibre curvature as a function of the length along the fibre, $l$, which is then useful for numerical simulations. Fig. S1 shows fibre shapes for $\Delta\theta$ ranging from zero to $\pi$ in both directions.

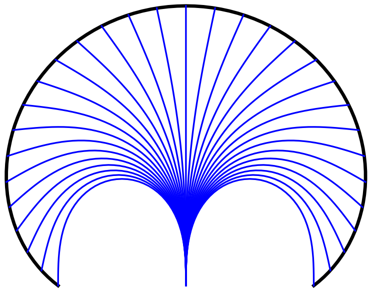

**Figure S1**: Fibre shapes corresponding to zero curvature at both ends for $\Delta\theta$ ranging from zero to $\pi$ in both directions. The curves were subsequently rotated so that the proximal end always points in the same direction (here vertically), which also corresponds to our experimental setup. The black curve marks the positions of the distal end for different $\Delta\theta$.

5. Simulation of the Refractive Index perturbations on imaging performance

Here we explore the influence of various types of refractive index perturbations on the imaging performance of the bent fibre. The simulation is analogous to that of the manuscript, i.e. we propagate through bent fibre the light fields that would lead to perfect foci in the straight fibre. These foci are used to image (raster scan) periodic sinusoidal gratings to reconstruct the contrast transfer function, which is then used to identify the resolution and estimate the resulting imaging capacity. The fibre features specifications of $\mathrm{GI}_{\mathrm{M}}^{2}$ and it is adiabatically bent to 90 degrees. The fibre's $n^2$ is considered as perfectly parabolic with a perturbation defined by a single Zernike polynomial. The polynomial is normalised so that $\int_0^R \int_0^{2\pi} \frac{r}{R^2} Z_m^n\left(\frac{r}{R}, \phi\right)\, \mathrm{d}r\, \mathrm{d}\phi = 1$, where $R$ is the radius of the fibre core. Its magnitude is varied by a multiplicative factor, ranging between $-10^{-3}$ and $10^{-3}$ (unitless as it describes changes to the $n^2$). The results are shown in Figure S2.
The first 'piston' $(Z_0^0)$ term has not been studied, as it will not affect the bending resilience (the effect is identical in straight and bent fibres, and it would be accounted for during the calibration). The behaviour of the lower orders agrees with intuitive expectations: The linear $n^2$ slant, perpendicular to the bending direction $(Z_1^{-1})$, has no effect as it only shifts the light in the $y$ direction. The linear $n^2$ slant, in the direction of the bending $(Z_1^1)$, has the same effect as the bending itself. While negative values add to the bending effect and push the propagating light towards the core-cladding boundary where it suffers from attenuation and coupling between modes, the positive values counter-act the effect and prevent the signals from coupling and losses. The parabolic term $(Z_2^0)$ is identical with the $n^2$ profile of the ideal fibre, its negative values thereby effectively increase the fibre's NA which leads to an increase in the imaging capacity (higher NAs are more immune to potential slant due to bending, the off-axis displacement of the potential well is smaller).

With higher orders, the observations exhibit a stark contrast between the aberrations of the even orders - antisymmetric with respect to the axis, and the odd orders - symmetric with respect to the axis), which follows the expectation derived above in Materials and Methods, Section 2.

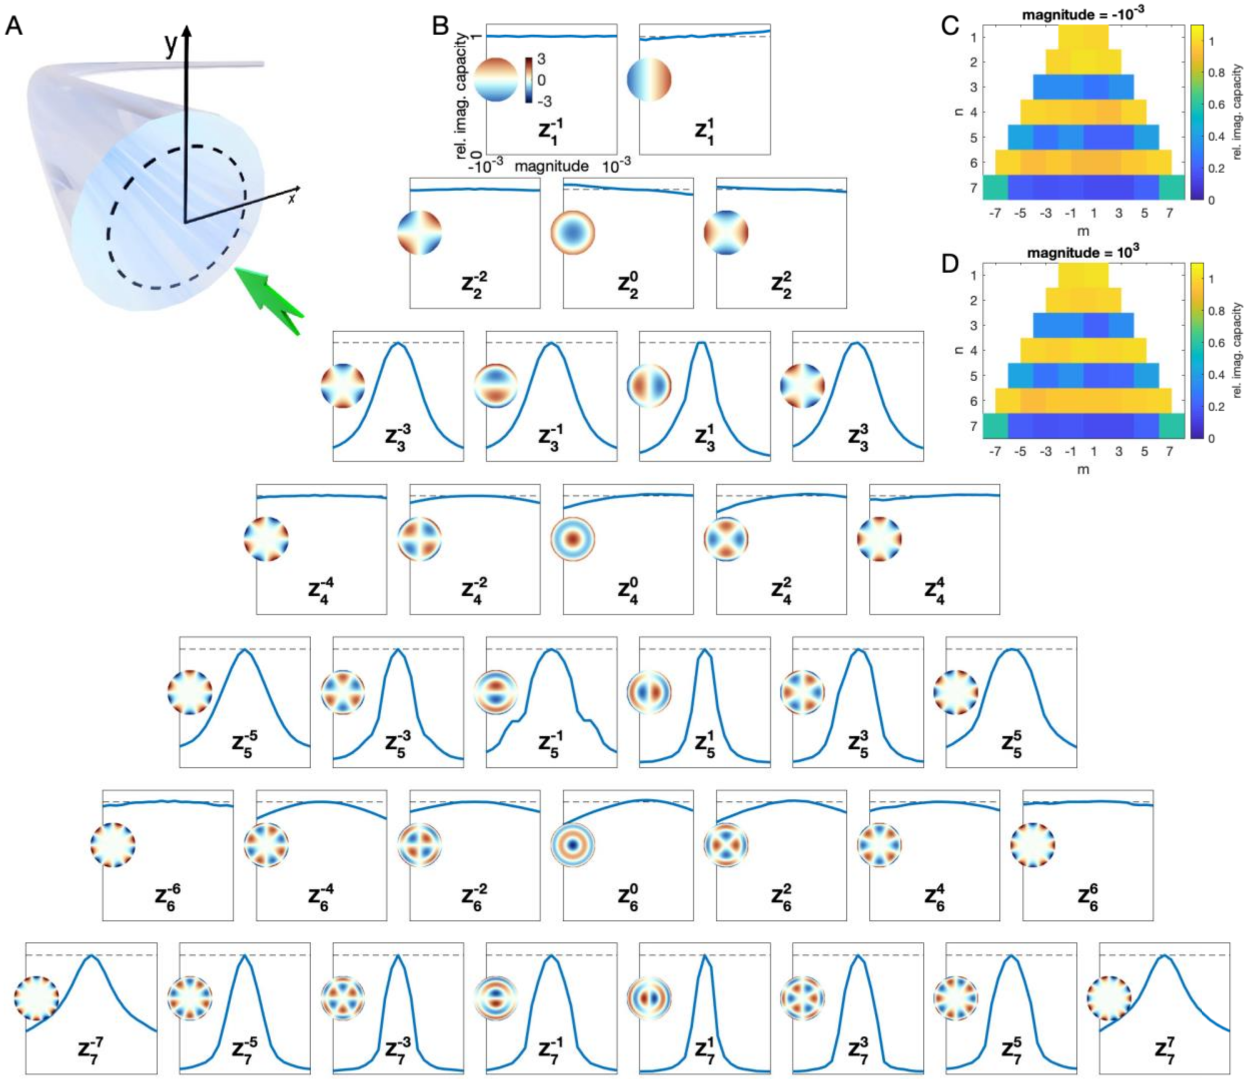


**Fig. S2.** Bending resilience of imaging for fibres featuring various aberrations in $n^2$ profile. **A**, The considered geometry of 34 mm long segment bent adiabatically to 90°. **B**, Relative imaging capacities (with respect to unperturbed fibre, core diameter of 50 μm, NA of 0.29) for aberrations described by Zernike polynomials, as functions of perturbation magnitude. **C** and **D**, Relative imaging capacities for the lowest and the highest refractive index aberration magnitude studied.

6. <u>Assessment of the Refractive Index of the used fibres</u>

Profiles of optical refractive index for the fibres utilised in this work in both experimental and simulation parts were obtained via IFA-100 Multiwavelength Optical Fiber Analyzer from Interfiber Analysis. By scanning the fibre probe under-test from the side, recording the relative phase and tomographic reconstruction methods, the device for optical refractive index profile measurements with claimed minimal detectable index fluctuations at the level of n=±0.0001. All measurements were carried out at a wavelength of 632nm, during tomographic imaging the fibre was rotated over 180° with steps of 5° [4,5]. The perturbations $\Delta n^2$ to perfectly parabolic profile of $n^2$, identified by this procedure, are summarized in Figs. S3 – S6, also isolating their antisymmetric and symmetric contributions.

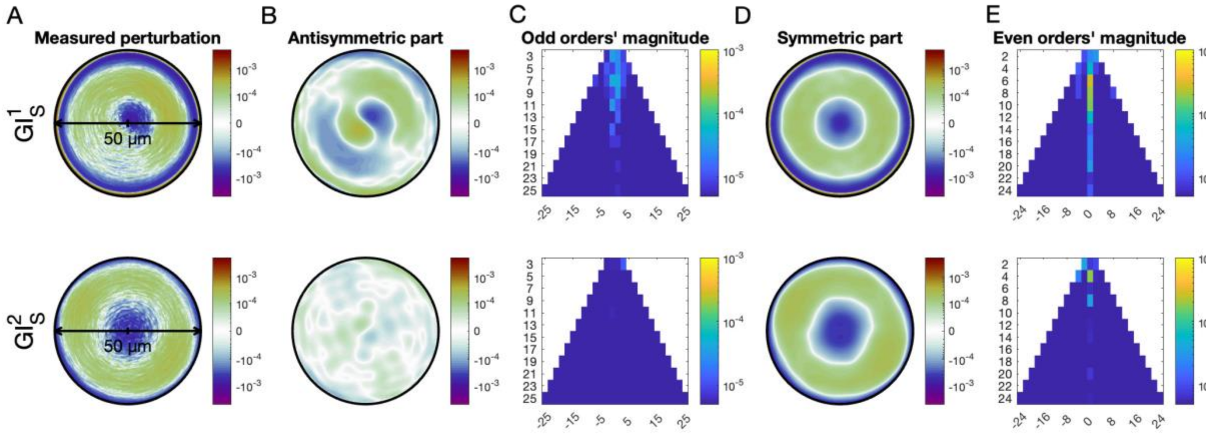


**Fig. S3.** Analysis of the refractive index profiles for GIS fibres. **A**, the difference of the measured $n^2$ and the ideal parabolic shape of the best fit acros the core area (diameter was set based on the manufacturer's specifications). Note the highly nonlinear false color representation shown in the colorbar. **B**, Antisymmetric part of the aberration composed of the odd orders of the Zernike polynomial basis. **C**, magnitude (absolute value) of the odd Zernike polynomials. **D**, Symmetric part of the aberration composed of the even orders of the Zernike polynomial basis. **E**, magnitude of the even Zernike polynomials.

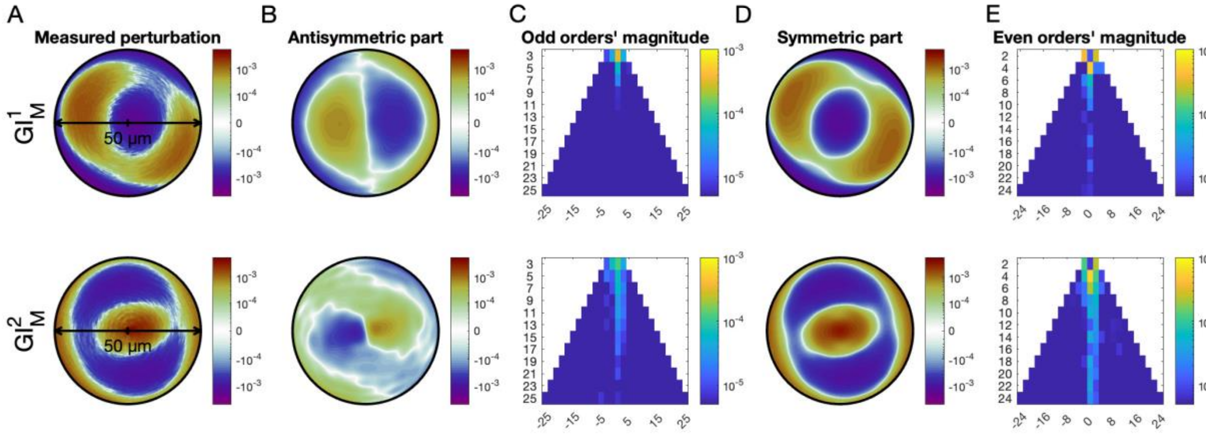


**Fig. S4.** Analysis of the refractive index profiles for GIM fibres. The organisation of the figure is identical to that of Fig. S3.

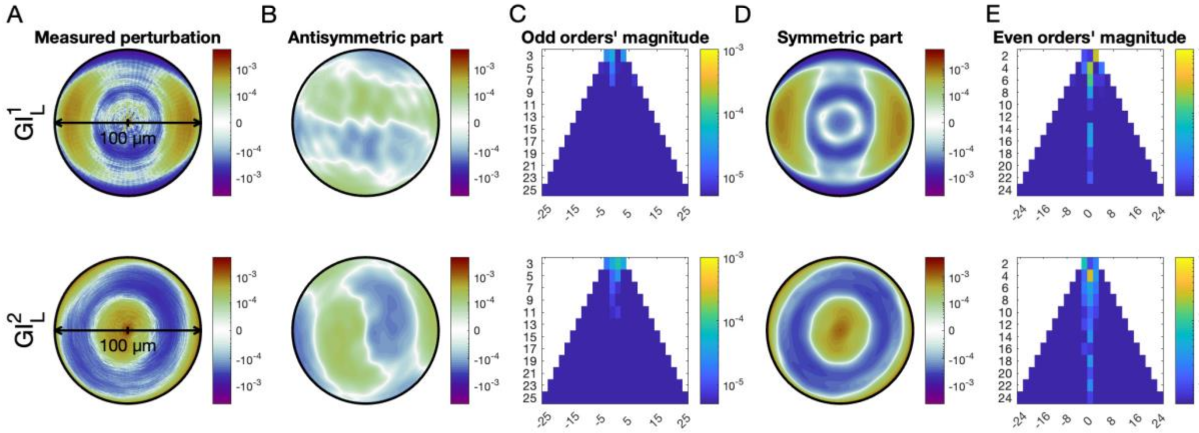

**Fig. S5.** Analysis of the refractive index profiles for $GI_L$ fibres. The organisation of the figure is identical to that of Fig. S3.

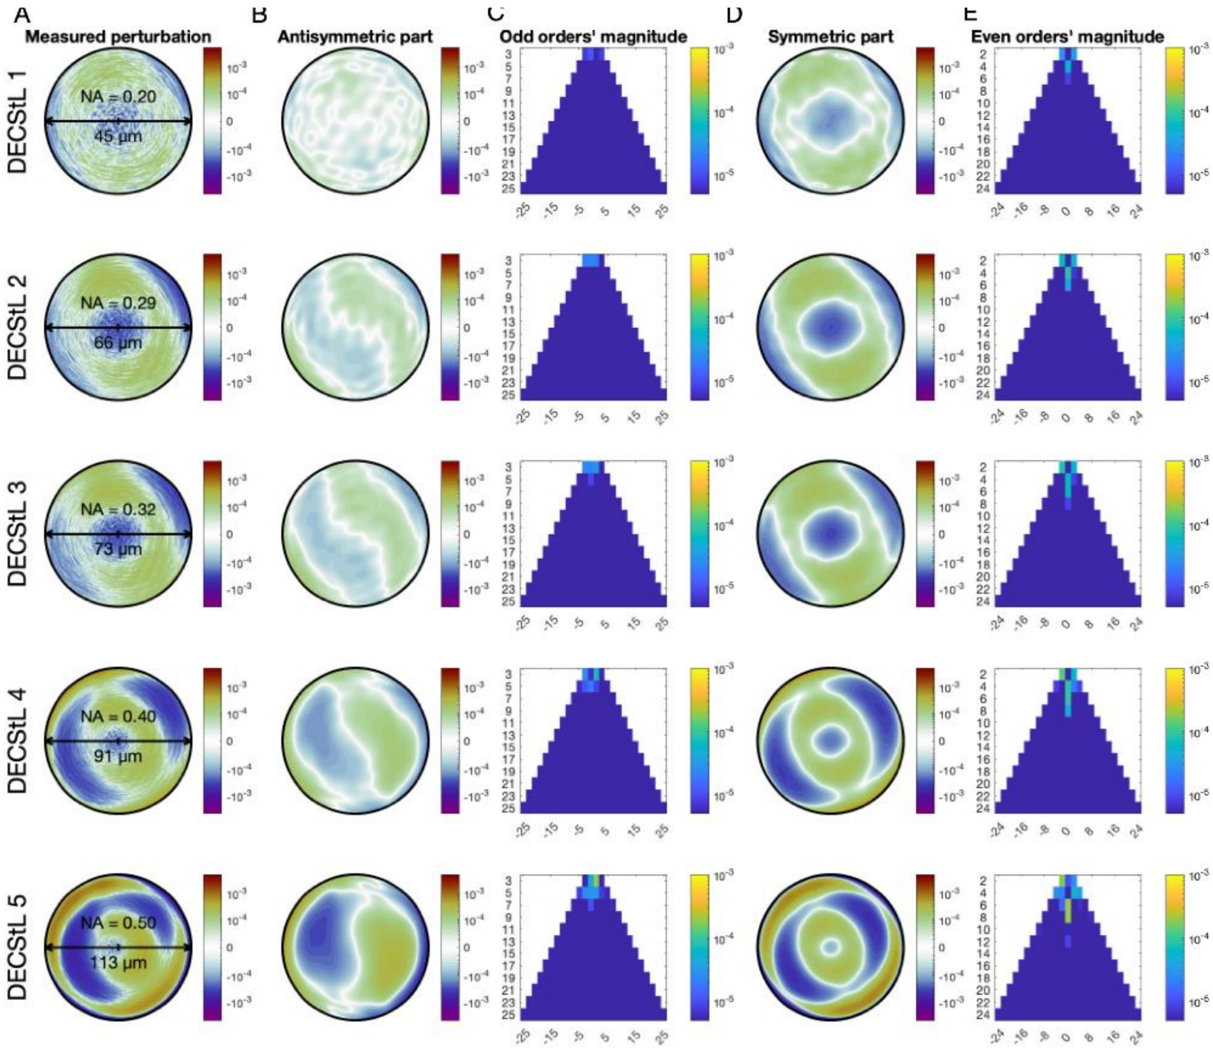


**Fig. S6.** Analysis of the refractive index profiles for the DECStL waveguide. The organisation of the figure is identical to that of Fig. S3. Individual rows shows different levels of truncation in virtual core size and NA, accordingly to Fig. 3.

7. <u>Simple metric for course bending resilience estimation</u>

As explained above in section 3, the influence of $\Delta n^2$ perturbation grows with the core radius $R$ and falls with the square of the NA. It is also the mainly the asymmetric part of $\Delta n^2$, causing the image degradation, as explained in section 2. Therefore, here we attempt to establish, whether and to what extent, the bending resilience can be estimated purely from the magnitude of this perturbation and the parameters of the fibre, without the necessity of the complete, and very computationally intensive mathematical algorithms used in this study. The simplest possible quantity would be the radius and NA regularised absolute value of $\Delta n^2$, averaged over the core of the fibre: $\langle\left|\frac{\Delta n^2 R}{NA^2}\right|\rangle$, which we refer to here as the bending resilience predictor (BRP). Figure S7 presents the relative decline of imaging capacity upon bending (the imaging capacity at $\epsilon = 90°$

over the imaging capacity at the initial straight state where calibration took place) against the corresponding BRP, for experimentally obtained as well as simulated results from our studies. As the 'rule of thumb' we can state that when BRP remains below the value of $5 \cdot 10^{-3} \mu m$ there is a good chance of bending resilience at least for applications involving imaging using 10s of cm long segments of fibre.

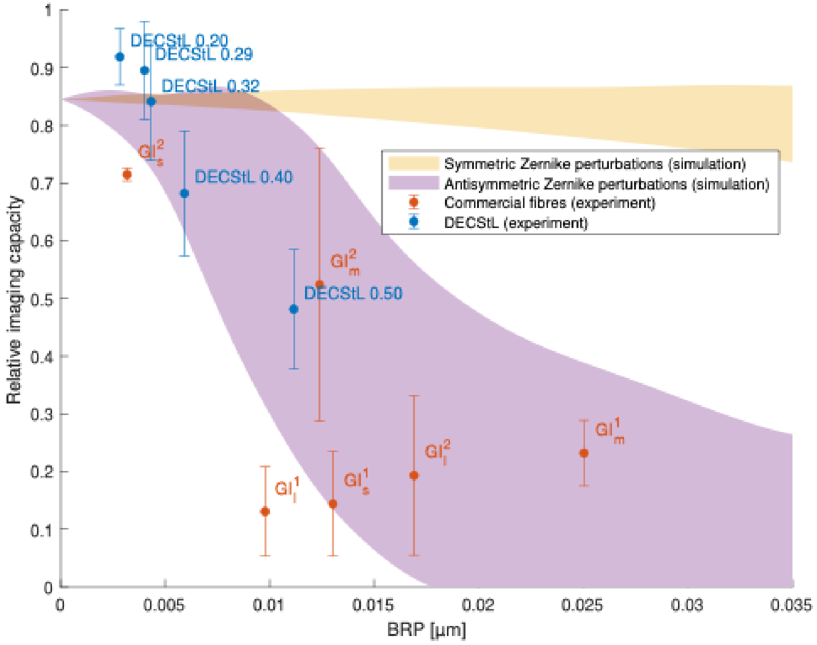


**Fig. S7.** Relative imaging capacity at $\epsilon = 90°$ as a function of bending resilience predictor. The shaded zones are single standard deviation wide confidence intervals obtained from simulations shown in Fig. S2. The points show the experimental data on commercial fibres and truncated DECStL, the corresponding error bars show the single standard deviation spread for the six roll orientations.

Note that the simulated data (for parameters of the $\mathrm{GI}_{\mathrm{M}}^{2}$ fibre) show the relative imaging capacity at zero BRP (no $\Delta n^2$perturbations) of $\approx 0.84$. This drop is caused by the transported light being displaced from the core due to the bending and a fraction of the signal, which penetrated to the cladding, has been decoupled. The same effect is present in all our fibres and it becomes stronger for shallower potential wells, i.e. smaller NA and larger core. This effect however does not occur in the truncated measurements of the DECStL waveguide as we can trim its core area and NA ony virtually at its extremities but not inside.

8. Fabrication of DECStL waveguides

The GRIN rods were fabricated by a silver-sodium based two-step ion exchange process in 125 µm rods of a patented glass composition[6]. For that, a polished cylindrical preform of this glass composition was fabricated by grinding and polishing before it was drawn to 125 µm diameter in a fibre drawing tower at temperatures of about 1000 °C. In a first ion exchange step, pieces of 60 mm length were immersed in a salt bath of a mixture of silver, sodium and potassium nitrate with a 20 % silver nitrate content. By this, around 90% of all sodium ions in the glass were replaced by silver ions leading to a high silver containing glass of homogenously increased refractive index of

about 1.64. In a second ion exchange step, these rods were subsequently placed in a sodium-potassium nitrate mixture to initiate a reverse out-diffusion process of silver ions from the surface of the glass rods, which are again replaced by sodium ions. This procedure results in the desired radial parabolic index profile of a numerical aperture of 0.5 and the maximum index at the centre of the rods.

9. Experimental Setup

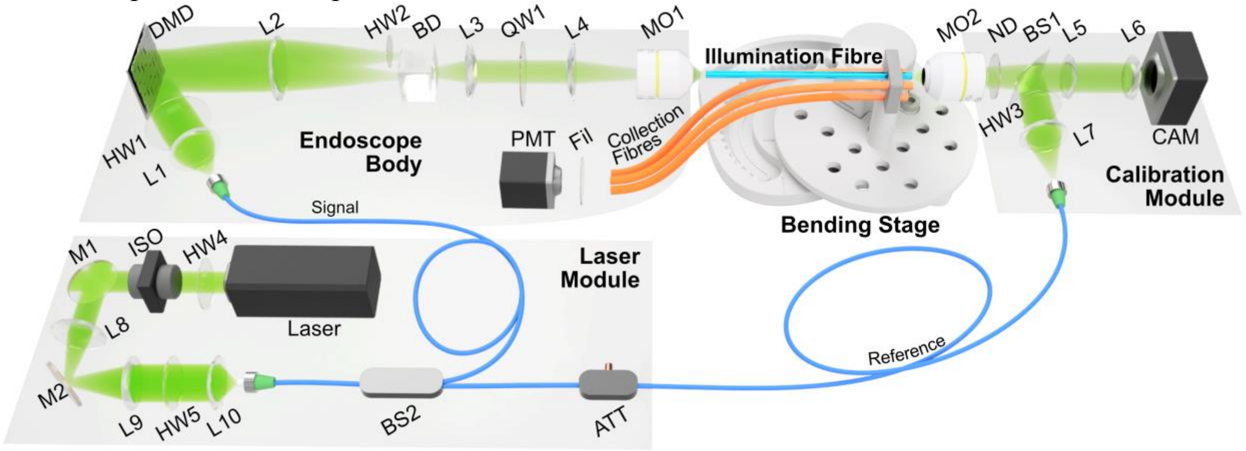


**Fig. S7.** Schematic representation of the experimental setup. Upon measurement of transmission matrix, the calibration module can be removed, and endoscope is ready for imaging. Specialised assemblies providing bending and rotational degrees of freedom for positioning fibre probes under test are presented in the Fig.S8 in greater details.

The linearly polarised light emitted by a single-frequency laser source (Coherent Sapphire 532 SF NX) at the 532 nm wavelength is coupled into the polarisation-maintaining fibre via lens assembly L8-10 and HW5 as depicted in Fig.S7. Subsequent fibre beamsplitter BS2 divides the coupled light into signal and reference arm with 99:1 ratio. The overall optical power in the system is controlled using HW4 placed before optical isolator ISO, while the power in the reference beam can be tuned independently by the MEMS-based fibre attenuator (ATT).
Two pairs of lenses, L2+L3 and L4+MO1, aligned in 4-f configuration, relay the DMD plane to the proximal fibre facet with appropriate demagnification. The demagnification of 80 times was chosen to closely match the linear size of the DMD active area (768 pixels x 13.69 µm pitch) to the core diameter of the largest probe employed in this study (DECStL, 125 µm). For the fibre types of a smaller core, the active area of the DMD was shrunk, allowing to match the core size and enable faster frame rates exceeding 30,000 FPS for the 50 µm core probes.
The input fields used for calibration are truncated plane waves coupled to the fibre at different incidence angles within the acceptance angle of the fibre defined by its NA. Such basis can be spatially resolved in the Fourier plane and represents an orthogonal grid of diffraction-limited foci, which can be steered across by changing the carrier frequency of the DMD gratings. In this work, two distantly spaced regions of the DMD Fourier plane were used to split illumination power into two beams. One of the beams passes through the half-wave plate HW2, changing polarisation to the orthogonal state and gets merged with another beam by polarisation beam displacer BD. Similarly to the previous work[7], this scheme allows gaining independent control over two orthogonal polarisation states of the light coupled to the fibre. The focal length of L2 and the

position of the beams in the Fourier plane are chosen to match the required beam separation of 4mm for the displacer BD.
The calibration module optical scheme consisting of microscope objective MO2 and a pair of lenses L5-6 is designed to image the far-field plane of the distal fibre facet onto a camera CAM. The reference beam delivered to the module by a polarisation maintaining fibre is collimated by the L7 and demagnified by the L5-L6 lens pair. Half-wave plate HW3 (Thorlabs WPMH10M-532) rotates the angle of polarisation of the phase reference beam, allowing to maximise interference contrast at CAM.

10. Design of the Bending Stage

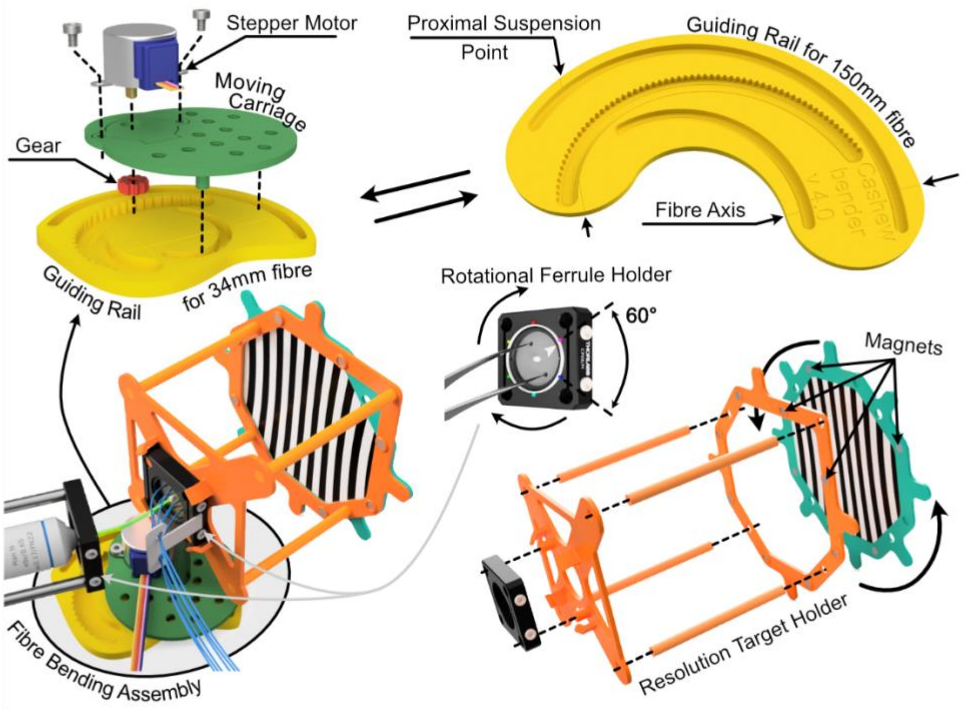


**Fig. S8.** 3D printed bending assemblies allowing for preforming bending, twisting deformations as well as imaging resolution Ronchi targets. Designs related to waveguide bending are available as supplementary Data S1.

11. Fibre length influence on bending resilience

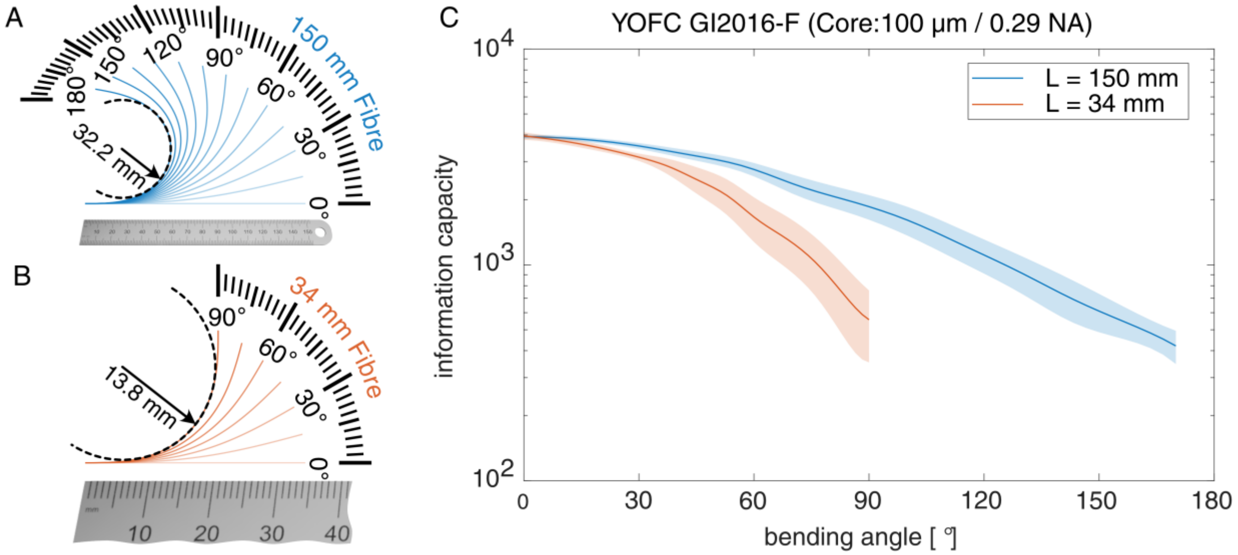


**Fig. S9.** Comparison of the under-bend imaging performance for two segments of the $\mathbf{GI_L^2}$ fibre (YOFC GI2016-F), which, however, differ in length. **A** and **B**, Bending layouts for both long (150mm) and short (34mm) fibre probes. **C**, Trends on bending resilience for two fibre pieces of different lengths confirm utilising longer fibres with restricted bending radii as a preferable way to minimise overall performance degradation. Error bars represent the standard deviation of imaging capacity resulted from the resolution target measurements taken for different rotational orientations of the fibre probe.

| Fibre ID | Manufacturer | Fibre Type | Profile | Core Size (µm) | Numerical aperture |
|---|---|---|---|---|---|
| SI | Thorlabs | FG050UGA | STEP | 50 ± 1 | 0.22± 0.02 |
| $GI_S^1$ | Corning | ClearCurve (OM5) | GRIN | 50 ± 2.5 | 0.200 ± 0.015 |
| $GI_S^2$ | Prismian Group | DRAKA WideCap (OM5) | GRIN | 50 ± 2.5 | 0.200 ± 0.015 |
| $GI_M^1$ | Prismian Group | DrakaElite 50/80um | GRIN | 50 ± 2 | 0.290 ± 0.015 |
| $GI_M^2$ | YOFC | GI2016-C | GRIN | 50±3 | 0.29 ± 0.02 |
| $GI_L^1$ | Prismian Group | DrakaElite 100/140um | GRIN | 100 ± 4 | 0.290 ± 0.015 |
| $GI_L^2$ | YOFC | GI2016-F | GRIN | 100 ± 3 | 0.29 ± 0.02 |
| DECStL | GrinTECH | custom | GRIN | ~125 | ~0.5 |

**Table S1:** List of the fibres utilised in the studies with a set of primary parameters specified by manufacturers.

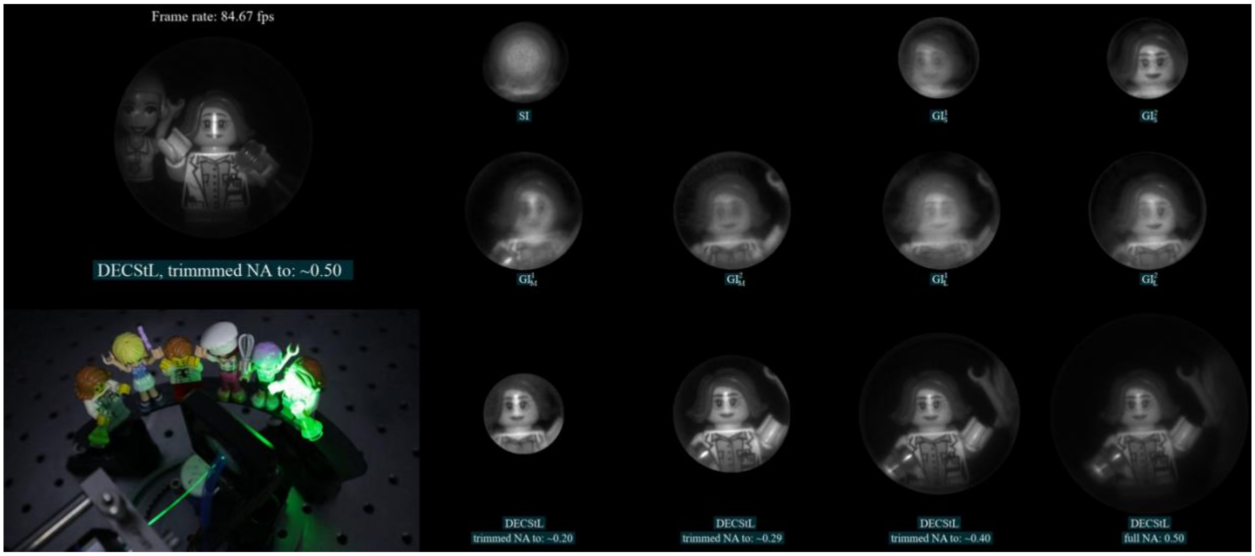


**Movie SM1**: Recordings of the scene during progressing bending deformation performed for the probes type under test. The probes of 34mm were bent from straight position to 90 degrees angle, which correspond to a maximum curvature radius of 13.8mm. For the fibres with significant difference of imaging performance on roll orientation both the worst as well as the best recordings are displayed.
Movie available from https://zenodo.org/records/18086670/files/SM1.mp4?download=1.

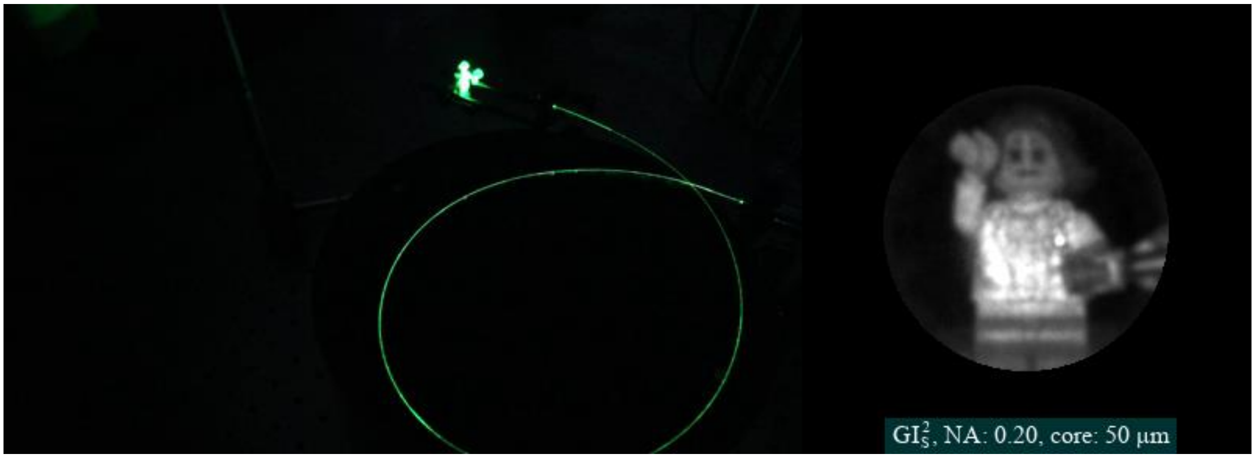


**Movie SM2**: Recording of the static scene containing a single Lego figurine while fibre experiencing pronounced bending deformations, mimicking fully flexible endoscope operation. The probe of $GI_5^2$ fibre type is 1m long. This fibre type demonstrated one of the best imaging performance resilience to bending deformation.
Movie available from https://zenodo.org/records/18086670/files/SM2.mp4?download=1.

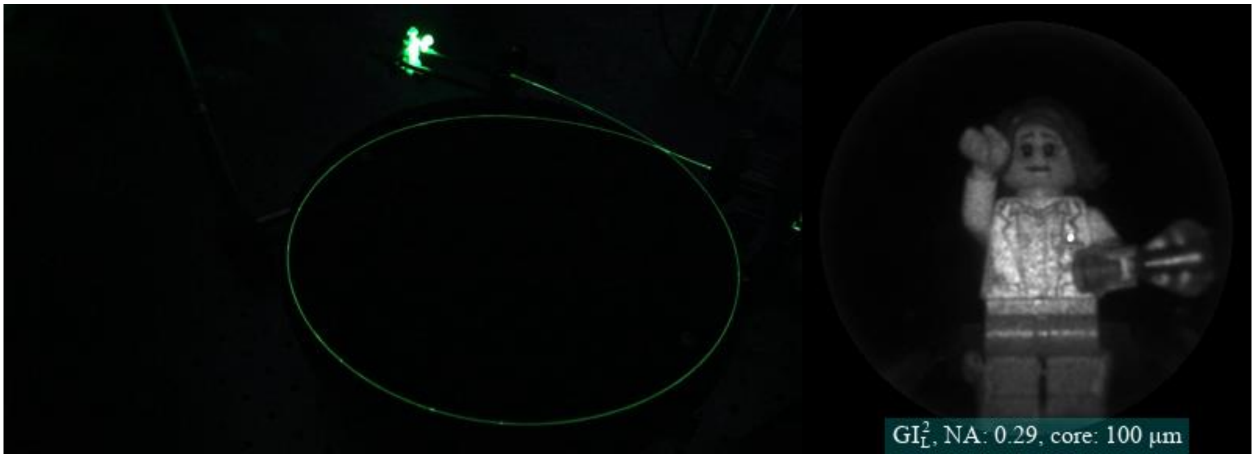


**Movie SM3:** Recording of the static scene containing a single Lego figurine while fibre experiencing pronounced bending deformations, mimicking fully flexible endoscope operation. The probe of $\mathbf{GI_L^2}$ fibre type is 1m long. This fibre type demonstrated one of the best imaging performance resilience to bending deformation. Movie available from https://zenodo.org/records/18086670/files/SM3.mp4?download=1.

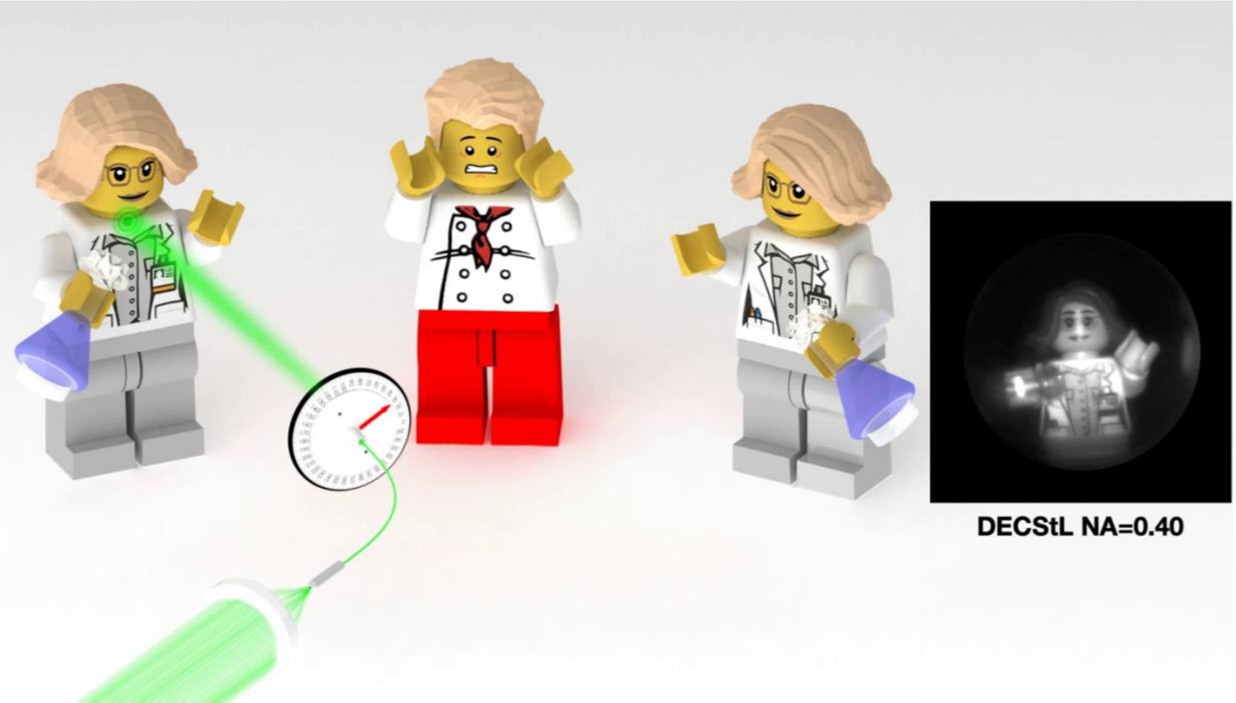


**Movie SM4:** Recordings of the scene during progressing twist deformation performed for the probes under test. Twisting of the distal end of the fibre probes was gradually changed from 0 to 30 degrees.
Movie available from https://zenodo.org/records/18086670/files/SM4.mp4?download=1.

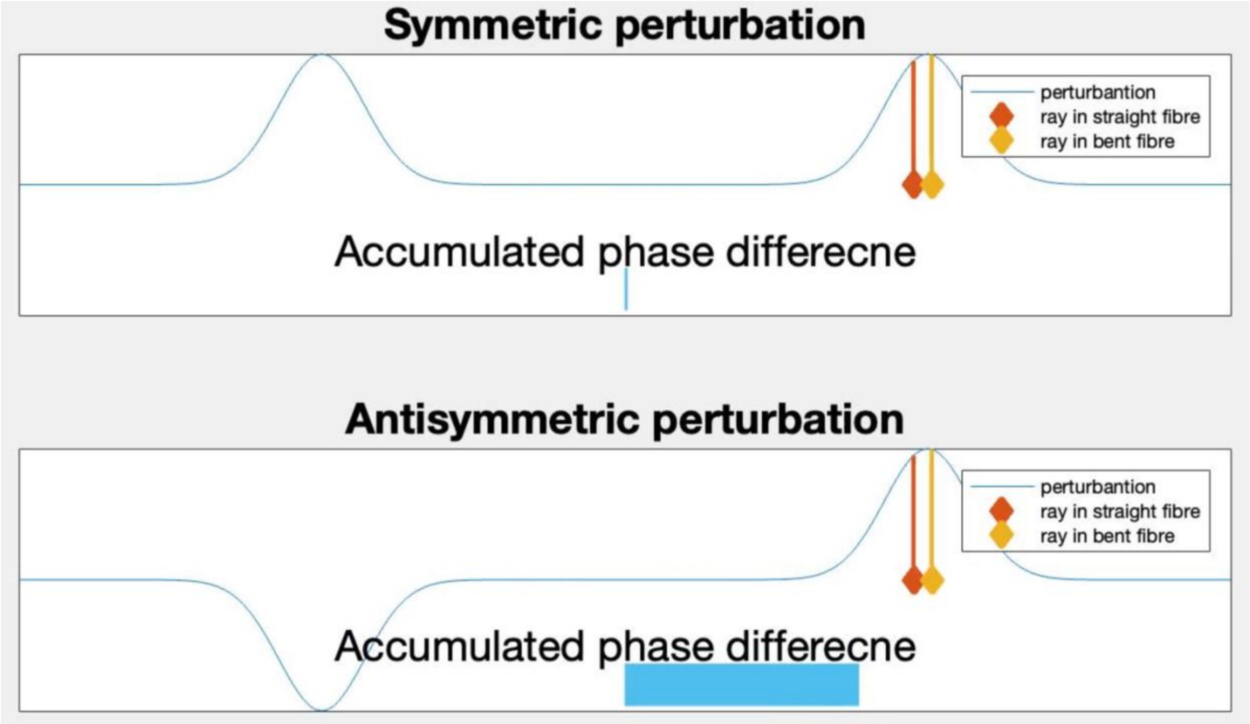


**Movie SM5:** The ‘naïve’ explanation of the contrasting bending resilience of fibres suffering from symmetric and asymmetric perturbations $\Delta n^2$, respectively. It derives from the fact that rays coupled into the fibre periodically visit the opposite sides of the core. When fibre is bent, the rays get displaced towards the outer side of the curved segment and are exposed to the influence of the perturbation causing a shift in the rays' phases. In case the perturbation is symmetric (even), its spatial derivative is odd, thereby the ray loses close to the same amount of phase on one side as what it has acquired on the opposite side previously, thereby cancelling both contributions. If the perturbation is, however, odd, its derivative is even, thereby the ray acquires similar amount of phase on both sides which accumulates along the whole propagation throughout the bend. Movie available from https://zenodo.org/records/18086670/files/SM5.mp4?download=1

**Data S1 (separate file - FibreBendingDesigns.zip): 3-D models for bending apparatus.**

The attached archive contains .stl files for 3D printed components used in this work for fibre bending. Files are named following nomenclature at Figure S8. Resource available from https://zenodo.org/records/18086670/files/FibreBendingDesigns.zip?download=1

**References:**

1. Snyder, A. W., Love, J. D. & others. *Optical waveguide theory*. vol. 175 (Chapman and hall London, 1983).
2. Flaes, D. E. B. *et al.* Robustness of light-transport processes to bending deformations in graded-index multimode waveguides. *Phys Rev Lett* **120**, 233901 (2018).
3. Landau, L. D., Lifshitz, E. M., Kosevich, A. M. & Pitaevskii, L. P. *Theory of elasticity: volume 7*. vol. 7 (Elsevier, 1986).
4. Yablon, A. D. Multi-wavelength optical fiber refractive index profiling by spatially resolved Fourier transform spectroscopy. *Journal of Lightwave Technology* **28**, 360–364 (2009).
5. Yablon, A. D. Multifocus tomographic algorithm for measuring optically thick specimens. *Opt Lett* **38**, 4393–4396 (2013).
6. Bernhard Messerschmidt *et al.* Alumino-boro-silicate glass and process to make crystal-free Gradient Index Lenses, *EP Patent*, EP1544176A2 (2004).
7. Gomes, A. D., Turtaev, S., Du, Y. & Čižmár, T. Near perfect focusing through multimode fibres. *Opt Express* **30**, 10645–10663 (2022).
